# Supplementary material for: FedBlock: A Blockchain Approach to Federated Learning against Backdoor Attacks
Source: arXiv:2411.02773 source file (2024-11-05)
Supplement: Supplementary file 1 [file additional.tex]

\section{Additional Work}\label{sec:additional}
\begin{document}

\vspace{1cm}

\end{document}
